# Supplementary material for: The Self-Improvement Paradox: Can Language Models Bootstrap Reasoning Capabilities without External Scaffolding?
Source: arXiv:2502.13441 source file (2025-02-19)
Supplement: Supplementary file 1 [file Appendix.tex]

% !TEX root = ./main.tex
%
%\appendix
\begin{appendices}

\section{Example Appendix}
\label{sec:appendix}

This is an appendix.

\end{appendices}
